# Supplementary material for: Controlling Large Language Models Through Concept Activation Vectors
Source: arXiv:2501.05764 source file (2025-01-10)
Supplement: Supplementary file 1 [file appendix.tex]

\section{Experiments detail}
